# Supplementary material for: Understanding the Role of the Projector in Knowledge Distillation
Source: arXiv:2303.11098 source file (2024-02-01)
Supplement: Supplementary file 1 [file supplementary.tex]

\newpage
% \section{Supplementary Material}

\subsection{Small capacity gap setting}
We ablate the importance of the repulsive force in the low-capacity gap setting, whereby we observe a much smaller performance improvement (see table \ref{table:repulsive_force}). This observation is likely attributed to the teacher no longer providing any sufficiently more discriminative representations to aid in the knowledge distillation process.

\begin{table}[htp]
    \centering
    % \parbox{.45\linewidth}{
    \centering
    \resizebox{\linewidth}{!}{%
    \begin{tabular}{llcc}
    \toprule
    Description & Repulsive force & acc@1 \\
    \midrule
    \stackengine{2pt}{Mean-square}{ \highlight{\footnotesize \textbf{no projection}} }{U}{c}{F}{T}{S} & $\lpnorm{z_s - z_t}_2^2$ & 71.08 \\
    % \midrule
    Mean-square & $\lpnorm{z_s - z_t}_2^2$ & 71.53 \\
    Batch-normalised & $\lpnorm{ \highlight{BN}(z_s) - \highlight{BN}(z_t) }_2^2$ & 71.34 \\
    Correlation & $\lpnorm{BN(z_s) \cdot BN(z_t) \highlight{- \mathbf{1}} }^2$ & 71.35 \\ 
    Higher-order & $\lpnorm{BN(z_s) \cdot BN(z_t) - \mathbf{1} }^\highlight{4}$ & 71.31 \\ 
    Soft maximum & $\highlight{log \sum} \lpnorm{BN(z_s) \cdot BN(z_t) - \mathbf{1} }^4$ & \textbf{71.63} \\ 
    \midrule
\end{tabular}
    }
    \caption{\textbf{Ablating the importance in the choice of metric function} using a ResNet34 and a ResNet18 student on the ImageNet dataset. The modifications are highlighted in \highlight{red}.}
    % and vanilla KD is provided as a reference
    \label{table:repulsive_force}
\end{table}

\subsection{Measure of translational equivariance}
In this section we provide more details on the proposed measure of translational equivariance and the motivation for its usage. In the cross inductive-bias distillation literature it is common to evaluate the effectiveness of a distillation pipeline through a measure of agreement between the student and the teacher~\cite{Touvron2021TrainingAttention, Ren2022Co-advise:Distillation}. We argue that this metric fails to encapsulate why one distillation method is more data efficient than another. We hypothesise that the most effective cross architecture distillation methods are those that transfer most of the inductive biases. To verify this claim, we introduce a measure of equivariance and show that a good distillation loss does indeed minimise this. For the convolution $\rightarrow$ transformer distillation setting, the most appropriate choice of measure is a measure of translational equivariance. This is because the teacher will have this equivariance explicitly enforced through the underlying convolutional layers, whereas the self-attention student will not. Recent works have shown that the self-attention layer can, in principle, learn the same operation as a convolution~\cite{Li2021CanConvolution}. The authors then show that injecting this bias will improve the data-efficiency, however, we show that this is not necessary since the bias can be learned implicitly through distillation.

Self-attention layers are known to be permutation equivariant. However, with the use of additive positional encodings, this restriction can be relaxed and can enable these layers to learn any arbitrary sequence-to-sequence function~\cite{Yun2020AreFunctions}. When we apply transformers to the vision domain, the tokens are provided as non-overlapping patches of the image. Thus, to perform a spatial translation on the sequence of tokens, we must first roll the sequence back to have the $H \times W$ dimensions in the same way in which we unrolled it at the input. The exact details can be seen in algorithm \ref{alg:equivariance}. Using this defined measure, we find that non-distilled transformers are over $15\times$ less equivariant than their distilled counterparts.

\begin{figure}[t]
\centering
\begin{minipage}[t]{0.9\linewidth}
% \begin{spacing}{0.7}
\begin{lstlisting}[basicstyle=\scriptsize\ttfamily, mathescape, language=Python, caption={Translational equivariance measure}, captionpos=t, numberbychapter=false,label={alg:equivariance}]
# x: Image representation B x N x C
# T: Spatial translation
# blk: Block of self-attention layers
def compute(x, T):
    # 14 x 14 patches
    h = 14
    w = 14
    b, n, c = x.shape

    # remove positional encodings
    xp = x[:, 2:]
    
    # roll token-dim into H x W dimensions
    xp = xp.transpose(1, 2).reshape(b, c, h, w)
    Tx = T(xp)

    # unroll H x W dimensions
    Tx = Tx.flatten(2).transpose(1,2)
    
    # add back the positional encodings
    Tx = torch.cat((x[:, 0:2], Tx), dim=1)

    # forward pass w/ and wo/ translation
    Fx = blk(x)
    FTx = blk(Tx)
    
    # remove position encoding
    Fxp = Fx[:, 2:]
    b, n, c = Fxp.shape
    
    Fxp = Fxp.transpose(1,2).reshape(b,c,h,w)
    TFxp = T(Fxp)
    TFxp = TFxp.flatten(2).transpose(1,2)
    
    # add back position encoding
    TFx = torch.cat((x[:, 0:2], TFxp), dim=1)
    
    return F.mse_loss(TFxp, FTx)
\end{lstlisting}
% \end{spacing}
\end{minipage}
\end{figure} 

% \vspace{-0.5em}
\subsection{Few-shot distillation experiments}
Due to the limited compute resources available, we were unable to perform some ablation experiments using the full ImageNet training data. To address this concern, and to avoid using a poor surrogate dataset (i.e. CIFAR100), we propose a more difficult few-shot distillation setting. In this setting, the models are still trained and evaluated on the large-scale ImageNet dataset, but with only a subset of the training data available. This results in the distillation objective being much more challenging. In all of these experiments we sample the same 20\% of images from each class to ensure the overall class balance is maintained.

% \vspace{-0.7em}
\subsection{Choice of batch size}
One of the main components in our distillation pipeline is the use of a joint batch normalisation for both the student and teacher features. Although this component does introduce a dependency on the batch size, we find that the performance is generally quite robust to its choice. Table \ref{table:batch} shows the student performance for various batch sizes, where we observe the best performance is achieved with the larger batch sizes. However, the performance degradation for the smaller batch sizes is within $0.3\%$. For the object detection experiments, we choose to normalise over the height and width dimensions, thus further relaxing the importance of batch size.

\begin{table}[H]
    \centering
    \resizebox{.65\linewidth}{!}{
\begin{tabular}{c|ccc}
    \toprule
    Batch size & 64 & 128 & 256 \\
    \midrule
    Accuracy (\%) & 71.36 & 71.41 & \textbf{71.63} \\
    \bottomrule
\end{tabular}
}
    \vspace{-0.5em}
    \caption{\footnotesize ImageNet ablation on batch size.}
    \label{table:batch}
\end{table}

\subsection{Additional logit losses}
For the main data efficient training of transformers experiment we use an additional distillation token alongside a logit distillation loss to compliment the feature distillation. However, for the CIFAR100 experiments, we do not use any additional logit distillation losses. In table \ref{table:cifar_logit} we show results with and without the DKD~\cite{Zhao2022DecoupledDistillation} loss. These results show that our feature distillation is complimentary logit distillation, leading to further improvements.

\begin{table}[H]
    \centering
    % \begin{small}
\setlength\tabcolsep{5pt}
\resizebox{.65\linewidth}{!}{
\begin{tabular}{c|cc}
    \toprule
    \belowrulesepcolor{mygrey}
    \rowcolor{mygrey} Teacher & ResNet32×4 & ResNet50 \\
    \belowrulesepcolor{mygrey}
    \rowcolor{mygrey} Student & ResNet8×4 & MobileNet-V2 \\
    \midrule
    Teacher & 79.42 & 79.34 \\ 
    Student & 72.50 & 64.60 \\ 
    \midrule
    KD & 73.33 & 64.60 \\ 
    CRD & 75.51 & 69.11 \\ 
    ReviewKD & 75.63 & 69.89 \\
    DKD & 76.32 & 70.35  \\
    
    % \midrule

    \aboverulesepcolor{myblue}
    \rowcolor{myblue} Ours & 76.55 & 71.53 \\   
    \aboverulesepcolor{myblue}
    \rowcolor{myblue} Ours + DKD & \textbf{76.95} & \textbf{71.75} \\   
    \aboverulesepcolor{myblue}

    \bottomrule
\end{tabular}
}
% \end{small}
    \vspace{-0.5em}
    \caption{\footnotesize CIFAR-100 with and without DKD.}
    \label{table:cifar_logit}
\end{table}

\subsection{Training dynamics for other architectures}
We further verify our observations on both the evolvement of singular values and the decorrelation of input-output features. For this we consider the cross-architecture setting using a CNN teacher and a ViT student model (see Figure \ref{fig:singular_decorrelation_joint}). 

\begin{figure}[H]
\centering
\resizebox{1.\linewidth}{!}{%
\includegraphics{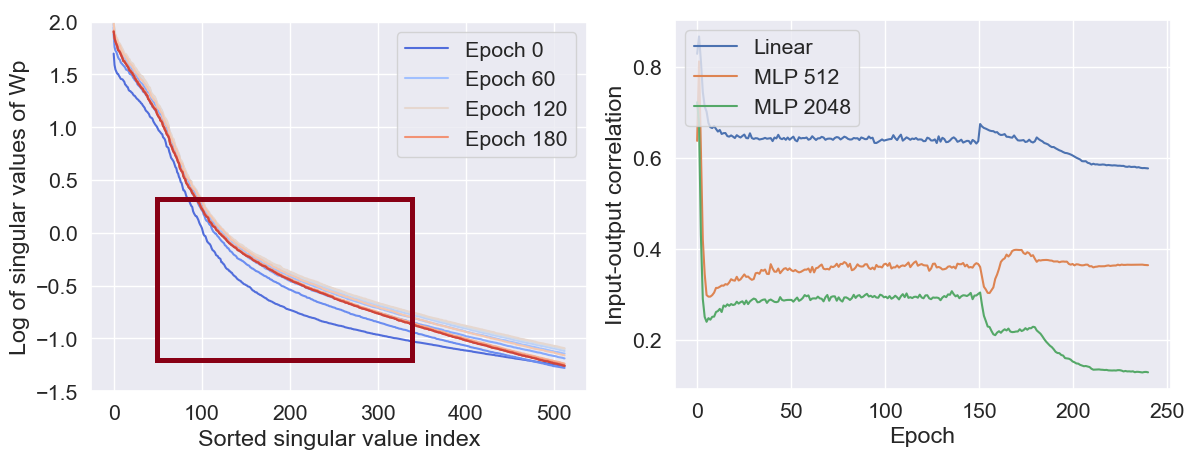}
}
\subfloat[Projector singular values]{\vspace{-6em}\hspace{.5\linewidth}}
\subfloat[Decorrelation of features]{\vspace{-6em}\hspace{.5\linewidth}}
\caption{Observing the same evolvement of singular values and decorrelation of input-output features in the cross-architecture setting.}
\label{fig:singular_decorrelation_joint}
\end{figure}

In general, the objective of feature distillation is to align the backbone features with the teacher, rather than solely aligning the projected features. This objective is imposed because we throw away the projector after training and so its learned representation would no longer be useful. This divergence of representations can happen when the projector has a sufficient capacity to learn a non-linear mapping between the two spaces (i.e. an MLP). Similarly, if the projector singular values are suppressed during training, the distillation loss will end up matching the teacher features in a much lower dimensional subspace, which will degrade the efficacy of distillation. These two observations motivate the need for both a \textbf{linear} projection and an appropriate normalisation scheme to encourage a diverse set of representations, which will avoid any rank collapse.

\subsection{Maximising the efficacy of distillation} 
In the previous section we discussed how suppressing singular values can degrade the efficacy of distillation. Here, we provide a more concrete explanation for this by showing that a low-rank projector does induce a loss in a lower-dimensional subspace. The rank of the projected features will be bounded by the rank of the projector:

\begin{align}
    &Rank(\mathbf{Z}_s\mathbf{W}_p) \leq \min(Rank(\mathbf{Z}_s), \overbrace{Rank(\mathbf{W}_p)}^{\text{Low-rank}})
\end{align}
\vspace{0.3em}

Thus, if the projector is low-rank then so too must be the projected features. The resulting distillation loss can now be expressed as follows:

\begin{align}
    \mathbf{Z}_s\mathbf{W}_p &= {\textstyle\sum}_{i}^r \sigma_i \mathbf{u}_i \mathbf{v}_i \text{, \;\; where $r$ is small} \nonumber \\
    \rightarrow \mathcal{L}_{distill} &= D\left({\textstyle\sum}_i^r \sigma_i \mathbf{u}_i \mathbf{v}_i, \mathbf{Z}_t\right),
\end{align}
\vspace{0.5em}

which is minimised when the projected features align with the the optimal low-rank approximation of $\mathbf{Z}_t$. This solution is suboptimal from the view of distillation. Since we wish to maximise the knowledge transfer, it is important for the projected features to have full-rank, which is encouraged using an appropriate normalisation scheme and a linear projection.

\subsection{Model Architectures}
In experiments, we use the following model architectures.
\begin{itemize}
    \item Wide Residual Network (WRN)~\cite{Zagoruyko2016WideNetworks}: WRN-$d$-$w$ represents wide ResNet with depth $d$ and width factor $w$.
\item resnet~\cite{He2015ResNetRecognition}: We use ResNet-d to represent CIFAR-style resnet with 3 groups of basic blocks, each with 16, 32, and 64 channels, respectively. In our experiments, resnet8x4 and resnet32x4 indicate a 4 times wider net- work (namely, with 64, 128, and 256 channels for each of the blocks).
    \item ResNet~\cite{He2015ResNetRecognition}: ResNet-d represents ImageNet-style ResNet with bottleneck blocks and more channels.
    \item MobileNetV2~\cite{Fox2018MobileNetV2:Bottlenecks}: In our experiments, we use a width multiplier of 0.5.
    \item vgg~\cite{Simonyan2015VeryRecognition}: The vgg networks used in our experiments are adapted from their original ImageNet counterpart.
    \item ShuffleNetV1~\cite{Zhang2018ShuffleNet:Devices}, ShuffleNetV2~\cite{Ma2018ShufflenetDesign}: ShuffleNets are proposed for efficient training and we adapt them to input of size 32x32.
\end{itemize}

\paragraph{Implementation Details.}
Both the ImageNet and CIFAR experiments follow the same training procedures as CRD~\cite{Tian2019ContrastiveDistillation}. However, for completeness, we choose to restate the details here. \\
\;\; For the CIFAR-100 experiments we use the SGD optimizer with an initial learning rate of 0.05, and with a decay of 0.1 every 30 epochs after the first 150 epochs until the last 240 epoch. For MobileNetV2, ShuffleNetV1 and ShuffleNetV2, we use a learning rate of 0.01 as this learning rate is optimal for these models in a grid search, while 0.05 is optimal for other models. \\
\;\; For the ImageNet experiments we train for 100 epochs with a 0.1 decay at epochs 30, 60, and 90. Further details are provided in the \textit{torchdistill} library. \\
\;\; Finally, for the data-efficient training of transformers, we use the same training schedule as DeIT~\cite{Touvron2021TrainingAttention}. This training pipeline uses the AdamW optimizer with Mixup, Cutmix and RandAugment. We choose a batch size of 512 on a single GPU. All our experiments are performed on a single NVIDIA RTX TITAN GPU with 24GB of memory.
